# Supplementary material for: A fluid bilayer phase in aqueous mixtures of fatty alcohol and cationic surfactant
Source: arXiv:1907.08779 source file (2019-07-20)
Supplement: Supplementary file 1 [file L_alpha_in_fatty_alcohols_SM.tex]

%% ****** Start of file apstemplate.tex ****** %
%%
%%
%%   This file is part of the APS files in the REVTeX 4.2 distribution.
%%   Version 4.2a of REVTeX, January, 2015
%%
%%
%%   Copyright (c) 2015 The American Physical Society.
%%
%%   See the REVTeX 4 README file for restrictions and more information.
%%
%
% This is a template for producing manuscripts for use with REVTEX 4.2
% Copy this file to another name and then work on that file.
% That way, you always have this original template file to use.
%
% Group addresses by affiliation; use superscriptaddress for long
% author lists, or if there are many overlapping affiliations.
% For Phys. Rev. appearance, change preprint to twocolumn.
% Choose pra, prb, prc, prd, pre, prl, prstab, prstper, or rmp for journal
%  Add 'draft' option to mark overfull boxes with black boxes
%  Add 'showkeys' option to make keywords appear
\documentclass[aps,prl,preprint,groupedaddress]{revtex4-1}
%\documentclass[aps,prl,preprint,superscriptaddress]{revtex4-2}
%\documentclass[aps,prl,reprint,groupedaddress]{revtex4-2}

% You should use BibTeX and apsrev.bst for references
% Choosing a journal automatically selects the correct APS
% BibTeX style file (bst file), so only uncomment the line
% below if necessary.
%\bibliographystyle{apsrev4-2}

\usepackage{graphicx} 

\begin{document}

% Use the \preprint command to place your local institutional report
% number in the upper righthand corner of the title page in preprint mode.
% Multiple \preprint commands are allowed.
% Use the 'preprintnumbers' class option to override journal defaults
% to display numbers if necessary
%\preprint{}

%Title of paper
\title{Supplemental Material \\
A fluid bilayer phase in aqueous mixtures of  fatty alcohol and cationic surfactant}

% repeat the \author .. \affiliation  etc. as needed
% \email, \thanks, \homepage, \altaffiliation all apply to the current
% author. Explanatory text should go in the []'s, actual e-mail
% address or url should go in the {}'s for \email and \homepage.
% Please use the appropriate macro foreach each type of information

% \affiliation command applies to all authors since the last
% \affiliation command. The \affiliation command should follow the
% other information
% \affiliation can be followed by \email, \homepage, \thanks as well.
%\author{}
%\email[]{Your e-mail address}
%\homepage[]{Your web page}
%\thanks{}
%\altaffiliation{}
%\affiliation{}

\author{Tiago Espinosa de Oliveira}
\affiliation{Institut Charles Sadron, CNRS and University of Strasbourg, rue du Loess, F-67034 Strasbourg cedex 2, France}
\affiliation{Universidade Federal do Rio Grande do Sul, Porto Alegre, Brazil}
  \author{Fabien Leonforte}
  \author{Luc Nicolas-Morgantini}
    \author{Anne-Laure Fameau}
  \author{Bernard Querleux}
\affiliation{L'Or\'eal Research and Innovation, France.}
\author{Fabrice Thalmann}
\author{Carlos M. Marques}
  \affiliation{Institut Charles Sadron, CNRS and University of Strasbourg, rue du Loess, F-67034 Strasbourg cedex 2, France}
%Collaboration name if desired (requires use of superscriptaddress
%option in \documentclass). \noaffiliation is required (may also be
%used with the \author command).
%\collaboration can be followed by \email, \homepage, \thanks as well.
%\collaboration{}
%\noaffiliation

\date{\today}

%\begin{abstract}
%\end{abstract}

% insert suggested keywords - APS authors don't need to do this
%\keywords{}

%\maketitle must follow title, authors, abstract, and keywords
\maketitle

We employ all-atom molecular dynamics simulations using the GROMACS~5.1.2 package~\cite{gro_manual}. We use the CHARMM-36 force field parameters~\cite{2004_mackerell,2010_klauda_pastor}  for C$_{16}$OH, C$_{18}$OH and  CTAC adapted from  DPPC (dioleoyl phosphatidyl choline, a common glycerophospholipid) and methanol molecules. All the systems were built using {\it packmol}~\cite{2003_martinez_martinez,2009_martinez_martinez}  and submitted to an energy minimization step using the steepest descent algorithm~\cite{1993_deift_zhou}, in order to relax the initial stresses. The system is submitted to a short thermalization simulation (1~ns) using the Berendsen thermostat and barostat~\cite{1984_berendsen_haak}, with a coupling constant of 0.5~ps at a temperature of 315~K and pressure 1~bar. The production simulations consisted of 100~ns runs with a varying temperature from 278 to 358~K. The temperature was controlled by a Nos\'e-Hoover thermostat~\cite{1984_nose,1985_hoover} with a coupling constant of 0.5~ps. Simulations were performed with a constant pressure set to 1~bar using the Parrinello-Rahman~\cite{1980_parrinello_rahman} semi-isotropic barostat with a coupling time of 2.0~ps. The long-range electrostatic interactions were handled  using the particle mesh Ewald (PME) method~\cite{1995_essmann_pedersen}. The interaction cutoff for non-bonded interactions was chosen equal to 1.2~nm. The time step for the simulations was set to 2~fs and the equations of motion were integrated using the leap-frog algorithm~\cite{1970_hockney}. All H-bond vibrations were constrained using the LINCS algorithm~\cite{1997_hess_fraaije}.

% If you have acknowledgments, this puts in the proper section head.
%\begin{acknowledgments}
% put your acknowledgments here.
%\end{acknowledgments}

% Create the reference section using BibTeX:
%\bibliography{fa}
%merlin.mbs apsrev4-1.bst 2010-07-25 4.21a (PWD, AO, DPC) hacked
%Control: key (0)
%Control: author (8) initials jnrlst
%Control: editor formatted (1) identically to author
%Control: production of article title (-1) disabled
%Control: page (0) single
%Control: year (1) truncated
%Control: production of eprint (0) enabled
%

\end{document}
